# Supplementary material for: Text Fact Transfer
Source: arXiv:2310.14486 source file (2023-10-23)
Supplement: Supplementary file 1 [file analogy.tex]

\begin{table*}[ht]
\small
\centering
\begin{tabularx}{\linewidth}{c | X }
\toprule
\textbf{Model} & \multicolumn{1}{c}{\textbf{Target Text}}  \\ \midrule
Ground Truth & mccartney plays piano.  \\ \midrule
Source Text & nicky hopkins plays pianist. \\ \midrule[1.5pt]
0-shot ModQGA & mccartney plays piano.  \\ \midrule
0-shot GPT & paul mccartney plays \textbf{\textcolor{red}{bassist}}.  \\ \midrule
0-shot GPT+Retr & mccartney plays \textbf{\textcolor{blue}{all the instruments on the song including pianist, drums, and bass}}.   \\ \midrule[1.5pt]
ModQGA-Sup & paul mccartney plays piano.  \\ \midrule
3-shot GPT & mccartney is \textbf{\textcolor{blue}{a musician}}.  \\ \midrule
10-shot GPT+Retr & \textbf{\textcolor{red}{nicky hopkins}} plays pianist \textbf{\textcolor{blue}{on the song}}.  \\ \midrule
LED & paul mccartney plays \textbf{\textcolor{blue}{bass}}.  \\ \midrule
BART+Retr & paul mccartney plays \textbf{\textcolor{blue}{drums}}.
 \\ \bottomrule
\end{tabularx}
\caption{\label{appendix:analogy} Sample target texts generated by baselines on Analogy with source topic Nicky Hopkins and target topic (Paul) McCartney. \textbf{\textcolor{red}{Red text}} indicates text that is factually incorrect. \textbf{\textcolor{blue}{Blue text}} indicates text that does not follow the style of the source text.}
\end{table*}
